# Supplementary material for: Variance Reduced Training with Stratified Sampling for Forecasting Models
Source: arXiv:2103.02062 source file (2021-06-11)
Supplement: Supplementary file 1 [file proof_old.tex]

\subsection{Proof to Theorem~\ref{theorem_groupingconvex}}
Since $f$ is strongly convex, we let
$\*\theta^*=\arg\min_{\*\theta}f(\*\theta)$. 
Since $f_{\mathcal{G}_i,j}, \forall i, j$ is convex, from Theorem 3.6 in \cite{gower2019sgd} we obtain
\begin{align}
    \|\nabla f_{\mathcal{G}_i,j}(\*\theta)-\nabla f_{\mathcal{G}_i,j}(\*\theta^*)\|^2\leq 2L[f_{\mathcal{G}_i,j}(\*\theta)-f_{\mathcal{G}_i,j}(\*\theta^*)-\nabla f_{\mathcal{G}_i,j}(\*\theta)^\top(\*\theta-\*\theta^*)], \hspace{1em}\forall i\in[1,B];j\in[1,|\mathcal{G}_i|]
\end{align}
Summing over $i,j$ and with $\nabla f(\*\theta^*)=0$, we obtain
\begin{align}
    \frac{1}{|\mathcal{G}|}\sum_{i=1}^{B}\sum_{j=1}^{|\mathcal{G}_i|}\|\nabla f_{\mathcal{G}_i,j}(\*\theta)-\nabla f_{\mathcal{G}_i,j}(\*\theta^*)\|^2\leq 2L(f(\*\theta)-f(\*\theta^*))
\end{align}
Let
\begin{align}
    \nabla f_{i_k^t,j_k^t}(\*\theta_k^t) = &\mathcal{O}_f(\*\theta_k^t)\\
    \nabla f_{i_k^t,j_k^t}(\*\theta_0^t) = &\mathcal{O}_f(\*\theta_0^t)
\end{align}
Taking the expectation with respect to $\*{\hat{\mu}}$ and then take the expectation with respect to $i_k^t$ and $j_k^t$, we obtain
\begin{align}
    & \mathbb{E}_{i_k^t,j_k^t}\mathbb{E}_{\*{\hat{\mu}}}\|\*v_k^t\|^2\\
    = & \mathbb{E}_{i_k^t,j_k^t}\mathbb{E}_{\*{\hat{\mu}}}\|\nabla f_{i_k^t,j_k^t}(\*\theta_k^t)-\nabla f_{i_k^t,j_k^t}(\*\theta_0^t)+\*{\hat{\mu}}\|^2\\
    = & \mathbb{E}_{i_k^t,j_k^t}\mathbb{E}_{\*{\hat{\mu}}}\|\nabla f_{i_k^t,j_k^t}(\*\theta_k^t)-\nabla f_{i_k^t,j_k^t}(\*\theta_0^t)+\nabla f(\*\theta_0^t)\|^2 + \mathbb{E}_{i_k^t,j_k^t}\mathbb{E}_{\*{\hat{\mu}}}\|\*{\hat{\mu}}-\nabla f(\*\theta_0^t)\|^2
\end{align}
the last equality holds due to the unbiasedness of $\*{\hat{\mu}}$:
\begin{align}
    \mathbb{E}_{\*{\hat{\mu}}}[\*{\hat{\mu}}] = \mathbb{E}_{\*{\hat{\mu}}}\left[\frac{1}{B}\sum_{i=1}^{B}\nabla f_{\mathcal{G}_i,j}(\*\theta_0^t)\right]=\frac{1}{B}\sum_{i=1}^{B}\mathbb{E}_{\*{\hat{\mu}}}\left[\nabla f_{\mathcal{G}_i,j}(\*\theta_0^t)\right]=\frac{1}{B}\sum_{i=1}^{B}\frac{1}{|\mathcal{G}_i|}\sum_{j=1}^{|\mathcal{G}_i|}\nabla f_{\mathcal{G}_i,j}(\*\theta_0^t)=\frac{1}{|\mathcal{G}|}\sum_{i=1}^{B}\sum_{j=1}^{|\mathcal{G}_i|}\nabla f_{\mathcal{G}_i,j}(\*\theta_0^t)
\end{align}
also since
\begin{align}
    \mathbb{E}_{\*{\hat{\mu}}}\|\*{\hat{\mu}}-\nabla f(\*\theta_0^t)\|^2 = & \mathbb{E}_{\*{\hat{\mu}}}\left\|\frac{1}{B}\sum_{i=1}^{B}\nabla f_{\mathcal{G}_i,j}(\*\theta_0^t)-\frac{1}{B}\sum_{i=1}^{B}\left[\frac{1}{|\mathcal{G}_i|}\sum_{m=1}^{|\mathcal{G}_i|}\nabla f_{i,m}(\*\theta_0^t)\right]\right\|^2\\
    = & \frac{1}{B^2}\mathbb{E}_{\*{\hat{\mu}}}\left\|\sum_{i=1}^{B}\nabla f_{\mathcal{G}_i,j}(\*\theta_0^t)-\sum_{i=1}^{B}\left[\frac{1}{|\mathcal{G}_i|}\sum_{m=1}^{|\mathcal{G}_i|}\nabla f_{i,m}(\*\theta_0^t)\right]\right\|^2\\
    = & \frac{1}{B^2}\sum_{i=1}^{B}\mathbb{E}_{\*{\hat{\mu}}}\left\|\nabla f_{\mathcal{G}_i,j}(\*\theta_0^t)-\left[\frac{1}{|\mathcal{G}_i|}\sum_{m=1}^{|\mathcal{G}_i|}\nabla f_{i,m}(\*\theta_0^t)\right]\right\|^2\\
    \leq & \frac{\sum_{i=1}^{B}\sigma_i^2}{B^2}
\end{align}
we use the unbiasedness in the third equality, then we obtain
\begin{align}
    & \mathbb{E}_{i_k^t,j_k^t}\mathbb{E}_{\*{\hat{\mu}}}\|\nabla f_{i_k^t,j_k^t}(\*\theta_k^t)-\nabla f_{i_k^t,j_k^t}(\*\theta_0^t)+\nabla f(\*\theta_0^t)\|^2 + \mathbb{E}_{i_k^t,j_k^t}\mathbb{E}_{\*{\hat{\mu}}}\|\*{\hat{\mu}}-\nabla f(\*\theta_0^t)\|^2\\
    %2
    \leq & 2\mathbb{E}_{i_k^t,j_k^t}\mathbb{E}_{\*{\hat{\mu}}}\|\nabla f_{i_k^t,j_k^t}(\*\theta_k^t)-\nabla f_{i_k^t,j_k^t}(\*\theta^*)\|^2 + 2\mathbb{E}_{i_k^t,j_k^t}\mathbb{E}_{\*{\hat{\mu}}}\|\nabla f_{i_k^t,j_k^t}(\*\theta_0^t)-\nabla f_{i_k^t,j_k^t}(\*\theta^*)+\nabla f(\*\theta_0^t)\|^2\\
    & +\frac{\sum_{i=1}^{B}\sigma^2_i}{B^2}\\
    %3
    \leq & 2\mathbb{E}_{i_k^t,j_k^t}\mathbb{E}_{\*{\hat{\mu}}}\|\nabla f_{i_k^t,j_k^t}(\*\theta_k^t)-\nabla f_{i_k^t,j_k^t}(\*\theta^*)\|^2+\frac{\sum_{i=1}^{B}\sigma^2_i}{B^2}\\
        & + 2\mathbb{E}_{i_k^t,j_k^t}\mathbb{E}_{\*{\hat{\mu}}}\|\nabla f_{i_k^t,j_k^t}(\*\theta_0^t)-\nabla f_{i_k^t,j_k^t}(\*\theta^*)-\mathbb{E}_{i_k^t,j_k^t}\mathbb{E}_{\*{\hat{\mu}}}[\nabla f_{i_k^t,j_k^t}(\*\theta_0^t)-\nabla f_{i_k^t,j_k^t}(\*\theta^*)]\|^2\\
    \leq & 2\mathbb{E}_{i_k^t,j_k^t}\mathbb{E}_{\*{\hat{\mu}}}\|\nabla f_{i_k^t,j_k^t}(\*\theta_k^t)-\nabla f_{i_k^t,j_k^t}(\*\theta^*)\|^2+\frac{\sum_{i=1}^{B}\sigma^2_i}{B^2}\\
        & + 2\mathbb{E}_{i_k^t,j_k^t}\mathbb{E}_{\*{\hat{\mu}}}\|\nabla f_{i_k^t,j_k^t}(\*\theta_0^t)-\nabla f_{i_k^t,j_k^t}(\*\theta^*)\|^2\\
    \leq & 4L[f(\*\theta_k^t)-f(\*\theta^*)+f(\*\theta_0^t)-f(\*\theta^*)] + \frac{\sum_{i=1}^{B}\sigma^2_i}{B^2}
\end{align}
We obtain
\begin{align}
    & \mathbb{E}[\|\*\theta_{k+1}^t-\*\theta^*\|^2|\*\theta_k^t]\\
    = & \|\*\theta_k^t-\*\theta^*\|^2 - 2\alpha\langle\*\theta_k^t-\*\theta^*, \mathbb{E}[\*v_k^t|\*\theta_k^t]\rangle+\alpha^2\mathbb{E}[\|\*v_k^t\|^2|\*\theta_k^t]\\
    \leq & \|\*\theta_k^t-\*\theta^*\|^2 - 2\alpha\langle\*\theta_k^t-\*\theta^*, \nabla f(\*\theta_k^t)\rangle+4\alpha^2L[f(\*\theta_k^t)-f(\*\theta^*)+f(\*\theta_0^t)-f(\*\theta^*)]+\frac{\alpha^2\sum_{i=1}^{B}\sigma^2_i}{B^2}\\
    \leq & \|\*\theta_k^t-\*\theta^*\|^2 - 2\alpha(f(\*\theta_k^t)-f(\*\theta^*))+4\alpha^2L[f(\*\theta_k^t)-f(\*\theta^*)+f(\*\theta_0^t)-f(\*\theta^*)]+\frac{\alpha^2\sum_{i=1}^{B}\sigma^2_i}{B^2}\\
    = & \|\*\theta_k^t-\*\theta^*\|^2 - 2\alpha(1-2\alpha L)(f(\*\theta_k^t)-f(\*\theta^*))+4\alpha^2L[f(\*\theta_0^t)-f(\*\theta^*)]+\frac{\alpha^2\sum_{i=1}^{B}\sigma^2_i}{B^2}
\end{align}
Using Option II and summing over the inner loop we obtain
\begin{align}
    & \mathbb{E}\|\*\theta_K^t-\*\theta^*\|^2 + 2\alpha(1-2\alpha L)K\mathbb{E}[f(\*\theta_0^{t+1})-f(\*\theta^*)]\\
    \leq & \mathbb{E}\|\*\theta_0^t-\*\theta^*\|^2 + 4LK\alpha^2\mathbb{E}[f(\*\theta_0^t)-f(\*\theta^*)] + \frac{\alpha^2\sum_{i=1}^{B}\sigma^2_iK}{B^2}\\
    = & \mathbb{E}\|\*\theta_0^t-\*\theta^*\|^2 + 4LK\alpha^2\mathbb{E}[f(\*\theta_0^t)-f(\*\theta^*)] + \frac{\alpha^2\sum_{i=1}^{B}\sigma^2_iK}{B^2}\\
    \leq & \frac{2}{\mu}\mathbb{E}[f(\*\theta_0^t)-f(\*\theta^*)] + 4LK\alpha^2\mathbb{E}[f(\*\theta_0^t)-f(\*\theta^*)] + \frac{\alpha^2\sum_{i=1}^{B}\sigma^2_iK}{B^2}\\
\end{align}
This implies
\begin{align}
    \mathbb{E}[f(\*\theta_0^{t+1})]-f(\*\theta^*) \leq & \left[\frac{1}{\mu\alpha(1-2\alpha L)K}+\frac{2\alpha L}{1-2\alpha L}\right]\mathbb{E}[f(\*\theta_0^t)-f(\*\theta^*)] + \frac{\alpha\sum_{i=1}^{B}\sigma^2_i}{2(1-2\alpha L)B^2}\\
    \leq & \rho^{T/K}\mathbb{E}[f(\*\theta_0^0)-f(\*\theta^*)] + \frac{\alpha\sum_{i=1}^{B}\sigma^2_i}{2(1-2\alpha L)(1-\rho)B^2}
\end{align}
where
\begin{align}
    \rho=\frac{1}{\mu\alpha(1-2\alpha L)K}+\frac{2\alpha L}{1-2\alpha L}
\end{align}
that completes the proof.

\subsection{Proof to Theorem~\ref{theorem_groupingnonconvex}}
We follow the proof technique of \cite{reddi2016stochastic} and define the following auxiliary sequence:
\begin{align}
    c_K =& 0\\
    c_k =& c_{k+1}(1+\alpha\beta+2\alpha^2L^2)+\alpha^2L^3\\
    \hat{\alpha} =& \alpha\left(1-\frac{c_{k+1}}{\beta}-\alpha L -2c_{k+1}\alpha\right)
\end{align}
where $\beta$ is a constant that will be assigned later.
Since $f$ is $L$-smooth, by the Taylor Theorem, in any outer loop $t$:
\begin{align}
    f(\*\theta_{k+1}^t) \leq f(\*\theta_{k+1}^t) - \langle \nabla f(\*\theta_k^t), \*\theta_{k+1}^t-\*\theta_k^t\rangle + \frac{L}{2}\|\*\theta_{k+1}^t-\*\theta_k^t\|^2
\end{align}
Take expectation on both sides, we obtain
\begin{align}
    \mathbb{E}[f(\*\theta_{k+1}^t)] \leq \mathbb{E}[f(\*\theta_{k}^t)] - \alpha\mathbb{E}\|\nabla f(\*\theta_k^t)\|^2 + \frac{\alpha^2L}{2}\mathbb{E}\|\*v_k^t\|^2
\end{align}
let
\begin{align}
    \Delta_k^t = \mathbb{E}[f(\*\theta_k^t) + c_k\|\*\theta_k^t-\*\theta_0^t\|^2]
\end{align}
and we obtain
\begin{align}
    \mathbb{E}\|\*\theta_{k+1}^t-\*\theta_0^t\|^2 = & \mathbb{E}\|\*\theta_{k+1}^t-\*\theta_k^t+\*\theta_k^t-\*\theta_0^t\|^2\\
    = & \mathbb{E}\|\*\theta_{k+1}^t-\*\theta_k^t\|^2 + \mathbb{E}\|\*\theta_k^t-\*\theta_0^t\|^2 + 2\mathbb{E}\langle \*\theta_{k+1}^t-\*\theta_k^t, \*\theta_k^t-\*\theta_0^t\rangle\\
    = & \alpha^2\mathbb{E}\|\*v_k^t\|^2 + \mathbb{E}\|\*\theta_k^t-\*\theta_0^t\|^2 - 2\alpha\mathbb{E}\langle \nabla f(\*\theta_k^t), \*\theta_k^t-\*\theta_0^t\rangle\\
    = & \alpha^2\mathbb{E}\|\*v_k^t\|^2 + \mathbb{E}\|\*\theta_k^t-\*\theta_0^t\|^2 + 2\alpha\mathbb{E}\left[\frac{1}{2\beta}\|\nabla f(\*\theta_k^t)\|^2+\frac{\beta}{2}\|\*\theta_k^t-\*\theta_0^t\|^2\right]
\end{align}
Then we obtain
\begin{align}
    \Delta_{k+1}^t \leq &  \mathbb{E}[f(\*\theta_k^t)] - \alpha\mathbb{E}\|\nabla f(\*\theta_k^t)\|^2 + \frac{\alpha^2L}{2}\mathbb{E}\|\*v_k^t\|^2 + \alpha^2c_{k+1}\mathbb{E}\|\*v_k^t\|^2\\
        & + c_{k+1}\mathbb{E}\|\*\theta_k^t-\*\theta_0^t\|^2 + 2\alpha c_{k+1}\mathbb{E}\left[\frac{1}{2\beta}\|\nabla f(\*\theta_k^t)\|^2+\frac{\beta}{2}\|\*\theta_k^t-\*\theta_0^t\|^2\right]\\
    \leq &  \mathbb{E}[f(\*\theta_k^t)] - \left(\alpha-\frac{\alpha c_{k+1}}{\beta}\right)\mathbb{E}\|\nabla f(\*\theta_k^t)\|^2 + \left(\frac{\alpha^2L}{2}+\alpha^2c_{k+1}\right)\mathbb{E}\|\*v_k^t\|^2\\
        & + c_{k+1}(1+\alpha\beta)\mathbb{E}\|\*\theta_k^t-\*\theta_0^t\|^2
\end{align}
We next bound the $\mathbb{E}\|\*v_k^t\|^2$:
\begin{align}
    \mathbb{E}\|\*v_k^t\|^2 = & \mathbb{E}\|\nabla f_{i_k^t,j_k^t}(\*\theta_k^t)-\nabla f_{i_k^t,j_k^t}(\*\theta_0^t)+\*{\hat{\mu}}\|^2\\
    = & \mathbb{E}\|\nabla f_{i_k^t,j_k^t}(\*\theta_k^t)-\nabla f_{i_k^t,j_k^t}(\*\theta_0^t)+\*{\hat{\mu}}-\nabla f(\*\theta_0^t)+\nabla f(\*\theta_0^t)\|^2\\
    = & \mathbb{E}\|\nabla f_{i_k^t,j_k^t}(\*\theta_k^t)-\nabla f_{i_k^t,j_k^t}(\*\theta_0^t)+\nabla f(\*\theta_0^t)\|^2 + \mathbb{E}\|\*{\hat{\mu}}-\nabla f(\*\theta_0^t)\|^2\\
    \leq & 2\mathbb{E}\|\nabla f_{i_k^t,j_k^t}(\*\theta_k^t)-\nabla f_{i_k^t,j_k^t}(\*\theta_0^t)+\nabla f(\*\theta_0^t)-\nabla f(\*\theta_k^t)\|^2 + 2\mathbb{E}\|\nabla f(\*\theta_k^t)\|^2 +  \frac{\sum_{i=1}^{B}\sigma_i^2}{B^2}\\
    \leq & 2\mathbb{E}\|\nabla f_{i_k^t,j_k^t}(\*\theta_k^t)-\nabla f_{i_k^t,j_k^t}(\*\theta_0^t)\|^2 + 2\mathbb{E}\|\nabla f(\*\theta_k^t)\|^2 +  \frac{\sum_{i=1}^{B}\sigma_i^2}{B^2}\\
    \leq & 2L^2\|\*\theta_k^t-\*\theta_0^t\|^2 + 2\mathbb{E}\|\nabla f(\*\theta_k^t)\|^2 + \frac{\sum_{i=1}^{B}\sigma_i^2}{B^2}
\end{align}
Push back we obtain
\begin{align}\label{UpdateDelta}
    \Delta_{k+1}^t \leq \Delta_k^t - \alpha\left(1-\frac{c_{k+1}}{\beta}-\alpha L -2c_{k+1}\alpha\right)\|\nabla f(\*\theta_{k}^t)\|^2 + \frac{\alpha^2\sum_{i=1}^{B}\sigma_i^2}{B^2}\left(\frac{L}{2}+c_{k+1}\right)
\end{align}
recall that
\begin{align*}
    c_K =& 0\\
    c_k =& c_{k+1}(1+\alpha\beta+2\alpha^2L^2)+\alpha^2L^3\\
    \hat{\alpha} =& \alpha\left(1-\frac{c_{k+1}}{\beta}-\alpha L -2c_{k+1}\alpha\right)
\end{align*}
Note that
\begin{align}
    c_0 = & c_K(1+\alpha\beta+2\alpha^2L^2)^K+\frac{(1+\alpha\beta+2\alpha^2L^2)^K-1}{\alpha\beta+2\alpha^2L^2}\alpha^2L^3\\
    = & \frac{(1+\alpha\beta+2\alpha^2L^2)^K-1}{\alpha\beta+2\alpha^2L^2}\alpha^2L^3
\end{align}
set the learning rate $\alpha=\frac{\delta}{L+\bar{\sigma}L\sqrt{T}}$, where $\bar{\sigma}^2=1/B\sum_{i=1}^{B}\sigma_i^2$,
$0<\delta<\frac{1}{3(e-1)}$ is a constant, set $\beta=\frac{L}{\bar{\sigma}^{\frac{1}{2}}T^{\frac{1}{4}}}$, then
\begin{align}
    & \alpha\beta+2\alpha^2L^2 \leq \frac{\delta}{\bar{\sigma}^{\frac{3}{2}}T^{\frac{3}{4}}} + \frac{2\delta^2}{\bar{\sigma}^2T} \leq \frac{2\delta}{\bar{\sigma}^{\frac{3}{2}}T^{\frac{3}{4}}}\\
    & \alpha^2L^3 \leq \frac{\delta^2L}{\bar{\sigma}^2T}
\end{align}
put it back to $c_0$ we obtain
\begin{align}
    c_0 = & \frac{(1+\alpha\beta+2\alpha^2L^2)^K-1}{\alpha\beta+2\alpha^2L^2}\alpha^2L^3\\
    = & \frac{(1+\alpha\beta+2\alpha^2L^2)^K-1}{2\bar{\sigma}^{\frac{1}{2}}T^{\frac{1}{4}}}\delta L
\end{align}
set $K=\left\lfloor \frac{\bar{\sigma}^{\frac{3}{2}}T^{\frac{3}{4}}}{2\delta}\right\rfloor$,
then
\begin{align}
    c_0 = & \frac{(1+\alpha\beta+2\alpha^2L^2)^K-1}{2\bar{\sigma}^{\frac{1}{2}}T^{\frac{1}{4}}}\delta L\\
    \leq & \frac{\left(1+\frac{2\delta}{\bar{\sigma}^{\frac{3}{2}}T^{\frac{3}{4}}}\right)^{\left\lfloor \frac{\bar{\sigma}^{\frac{3}{2}}T^{\frac{3}{4}}}{2\delta}\right\rfloor}-1}{2\bar{\sigma}^{\frac{1}{2}}T^{\frac{1}{4}}}\delta L\\
    \leq & \frac{\delta L(e-1)}{2\bar{\sigma}^{\frac{1}{2}}T^{\frac{1}{4}}}
\end{align}
since $c_k$ is decreasing, we obtain
\begin{align}
    \hat{\alpha} = &  \alpha\left(1-\frac{c_{k+1}}{\beta}-\alpha L -2c_{k+1}\alpha\right)\geq  \alpha\left(1-\frac{c_0}{\beta}-\alpha L -2c_0\alpha\right)
\end{align}
let $\delta$ fulfills the following criterion:
\begin{align}
    \frac{c_0}{\beta} = \frac{\delta (e-1)}{2} \leq & \frac{1}{6}\\
    \alpha L \leq  & \frac{1}{6}\\
    2c_0\alpha =\frac{2\alpha\delta L^2(e-1)}{2\bar{\sigma}T^{\frac{1}{4}}}\leq  & \frac{1}{6}
\end{align}
we obtain
\begin{align}
    \delta \leq \frac{1}{3(e-1)}
\end{align}
then
\begin{align}
    \hat{\alpha}\geq\frac{\alpha}{2}
\end{align}
Put it back to Equation~(\ref{UpdateDelta}), and telescope over $k$ and $t$ we obtain
\begin{align}
    \frac{1}{T}\sum_{t=0}^{T/K-1}\sum_{k=0}^{K-1}\mathbb{E}\|\nabla f(\*\theta_k^t)\|^2 \leq &  \frac{2(f(\*\theta_0^0)-f^*)}{T\alpha} + \frac{2\alpha\sum_{i=1}^{B}\sigma_i^2}{B^2}\left(\frac{L}{2}+\frac{\delta L^2(e-1)}{2\bar{\sigma}T^{\frac{1}{4}}}\right)\\
    \leq & \frac{2\bar{\sigma}}{B\sqrt{T}} + \frac{2(f(\*\theta_0^0)-f^*)\bar{\sigma}L}{\sqrt{T}} + \frac{2(f(\*\theta_0^0)-f^*)L}{T}\\
    = & \frac{2\sqrt{B^{-1}\sum_{i=1}^{B}\sigma_i^2}}{B\sqrt{T}} + \frac{2(f(\*\theta_0^0)-f^*)\sqrt{B^{-1}\sum_{i=1}^{B}\sigma_i^2}L}{\sqrt{T}} + \frac{2(f(\*\theta_0^0)-f^*)L}{T}
\end{align}
that completes the proof.
